# Supplementary material for: From Pixels to Legs: Hierarchical Learning of Quadruped Locomotion
Source: arXiv:2011.11722 source file (2020-11-23)
Supplement: Supplementary file 1 [file supplemental.tex]

\documentclass{article}

\usepackage{corl_2020} % Use this for the initial submission.

\usepackage{graphicx}
\graphicspath{{figures/}}
\usepackage[export]{adjustbox}
\usepackage{caption}
\usepackage{subcaption}
\usepackage{wrapfig}
\usepackage{algorithm}
\usepackage[noend]{algpseudocode}
\usepackage{setspace}
\usepackage{hyperref}
\usepackage{tikz}
\usetikzlibrary{positioning,shapes}
\usepackage{bm}
\usepackage{xcolor}
\usepackage{siunitx}
\usepackage{balance}
\usepackage{booktabs}
\usepackage{amsmath, amssymb}
\usepackage{subcaption}
\usepackage[percent]{overpic}
\usepackage[textsize=scriptsize,textwidth=1cm]{todonotes}

%\DeclareMathOperator{\dim}{dim}

% \title{From Pixels to Legs: \\Hierarchical Learning of Quadruped Locomotion}

% The \author macro works with any number of authors. There are two
% commands used to separate the names and addresses of multiple
% authors: \And and \AND.
%
% Using \And between authors leaves it to LaTeX to determine where to
% break the lines. Using \AND forces a line break at that point. So,
% if LaTeX puts 3 of 4 authors names on the first line, and the last
% on the second line, try using \AND instead of \And before the third
% author name.

% NOTE: authors will be visible only in the camera-ready (ie, when using the option 'final'). 
% 	For the initial submission the authors will be anonymized.

% \author{
%   Deepali Jain \\
%   Robotics at Google \\
%   \texttt{jaindeepali@google.com}
%   \And
%   Atil Iscen \\
%   Robotics at Google \\
%   \texttt{atil@google.com}
%   \And
%   Ken Caluwaerts \\
%   Robotics at Google \\
%   \texttt{kencaluwaerts@google.com}
% }

\begin{document}
% \maketitle

\input{sections/robot_transfer}

\bibliography{references}
\end{document}
